# Supplementary material for: Clover: Closed-Loop Verifiable Code Generation
Source: arXiv:2310.17807 source file (2024-11-16)
Supplement: Supplementary file 2 [file appendix_pseudocode.tex]

% Algorithm~\ref{algo:consistency-check} shows pseudocode for our implementation of \sys consistency checking.

% \begin{algorithm}[H]
%         \caption{Consistency Check ($k=1$) in \sys \label{algo:consistency-check}}
%         \begin{algorithmic}
% \Require Docstring $d$, annotation $a$, code $c$.
% \Ensure $True/False$

% \State

% \Comment{annotation soundness}
% \If{Dafny failed to verify $a, c$} 
%     \State \textbf{Return} $False$
% \EndIf


% \Comment{annotation completeness}
% \State Set number of tries $m=3$ 
% \State $p = False$
% \For{$i$ = 1 to $m$}
%     \State Call GPT-4 to generate code $c'$ from $a$ and feedbacks.
%     \If{$c'$ successfully compiles}
%         \State{break}
%     \EndIf
% \EndFor
% \If{$c'$ is not equivalent to $c$}
%     \State \textbf{Return} $False$
% \EndIf
% \Comment{doc2code}
% \For{$i$ = 1 to $m$}
%     \State Call GPT-4 to generate code $c'$ from $d$ and feedbacks.
%     \If{$c'$ successfully compiles}
%         \State{break}
%     \EndIf
% \EndFor
% \If{$c'$ is not equivalent to $c$}
%     \State \textbf{Return} $False$
% \EndIf
% \Comment{code2doc}
% \For{$i$ = 1 to $m$}
%     \State Call GPT-4 to generate docstring $d'_i$ from $c$.
% \EndFor
% \If{all $d'_i$ are not equivalent to $d$}
%     \State \textbf{Return} $False$
% \EndIf

% \Comment{doc2anno}
% \For{$i$ = 1 to $m$}
%     \State Call GPT-4 to generate annotation $a'$ from $d$ and feedbacks.
%         \If{$a'$ successfully compiles}
%         \State{break}
%     \EndIf
% \EndFor
%     \If{$a'$ is not equivalent to $a$}
%         \State \textbf{Return} $False$
%     \EndIf
% \Comment{anno2doc}
% \For{$i$ = 1 to $m$}
%     \State Call GPT-4 to generate docstring $d'$ from $a$.
% \EndFor
% \If{all $d'$ are not equivalent to $d$}
%     \State \textbf{Return} $False$
% \EndIf        
% \State \textbf{Return} $True$
% \end{algorithmic}
%     \end{algorithm}
